# Supplementary material for: JIGGLE: An Active Sensing Framework for Boundary Parameters Estimation in Deformable Surgical Environments
Source: arXiv:2405.09743 source file (2024-05-16)
Supplement: Supplementary file 2 [file appendix_copy_2_2_642pm.tex]

    % As discussed goal is minimizing entropy of the belief distribution
    % Computationally expensive, prone to local minima 
    % Choose the heuristic of displacement to try to get around this
    % To justify this we need to derive the relationship between displacement of the tissue surface and the the change in entropy. 
    % We organize this section as follows: We will first start by showing the relationship between entropy and the jacobian of the PBD simulator $\beljacob$ with respect to the boundary constraint parameter $b$. We will then derive the jacobian of the PBD simulator and show its relationship to displacement. Finally we will combine these two derivations to show how our heuristic choice of uncertainty weighted displacement reduces entropy. 

    % \subsubsection{Entropy} We first start by analyzing the equation for entropy as a function of our actions. 

    %     % The objective is to minimize the entropy of the belief distribution. 
%     % undertake the task of deriving the relationship between the displacement of the tissue surface and the corresponding change in entropy.

\newpage
\section{Appendix}
\subsection{Relationship Between Uncertainty-Weighted Displacement (UWD) and Boundary Entropy} \label{appendix:relationship_displacement_entropy}
\flnotehighlight{ 
    \textbf{
    \vspace{-0.4em}
    \begin{proposition}
        The active sensing objective of maximizing the uncertainty-weighted deformation displacement, i.e.,
            $\weighteddeform$ in Eq. \ref{eqn:uncertain_weighted_displacement},
        is designed to decrease the entropy $\entropy(\mathbf{b})$ of boundary estimation and uncovering more unknown information. That is,
            \begin{equation} \label{eqn:displacement_vs_entropy}
                \begin{split}
                   \max \weighteddeform \propto  \min \entropy(\mathbf{b})
                \end{split}
            \end{equation}
    \end{proposition}
    \vspace{0.4em}
    }
}
\flnote{
    In this section we present the above proposition, and provide a proof tying the relationship between the UWD, i.e., $\weighteddeform$, of the tissue particles from their initial position, and the reduction in boundary entropy $\entropy(\mathbf{b})$. To achieve this, we establish a connection via the observation Jacobian $\beljacob = \frac{\partial \obsmodel}{\partial \bel}$ defined by EKF in Eq. \ref{eqn:kalman_jacobians}.
}
\flnote{
\subsubsection{\textbf{Boundary Entropy Regarding the Observation Jacobian}}
    % ref: https://gregorygundersen.com/blog/2020/09/01/gaussian-entropy/
    As defined in Eq. \ref{eqn:kalman_entropy}, it is evident that the entropy $\entropy(\mathbf{b})$ is directly proportional to the determinant of the covariance matrix outputted by the Extended Kalman Filter (EKF) estimator. 
    % In our context, the covariance matrix of noises, $\motioncov_{t}, \obscov_{t}$, is a pre-determined constant that remains independent of the estimation. For simplification in the subsequent derivations, we denote this constant as $c_1 = \motioncov_{t}$, $c_2 = \obscov_{t}$.
    Since $\Sigmab_{t|t}, \motioncov_{t}, \obscov_{t}$ are all positive semi-definite covariance matrices, they allow the following factorization: 
    % ref1: https://stats.stackexchange.com/questions/632620/covariance-matrix-square-root
    % ref2: https://stats.stackexchange.com/questions/256422/meaning-of-square-root-of-covariance-precision-matrices
    \begin{equation}
        \begin{split}
            \Sigmab_{t+1|t} & = \Sigmab_{t|t} + \motioncov_{t} = \Sigmab^{\frac{1}{2}} \Sigmab^{\frac{1}{2}}
        \end{split}
    \end{equation}
    Combining this fact with the Extended Kalman Filter (EKF) equations as defined in Eq. \ref{eqn:predict_step} and \ref{eqn:update_step}, and for the sake of simplicity, neglecting the subscripts of observation Jacobian $\beljacob_{t+1}$ and Kalman gain $\kalmangain_{t+1}$, we obtain:
    \begin{equation}
        \label{eqn:entropy_}
        \begin{split}
            \entropy 
            & \propto \Big| \Sigmab_{t+1|t+1} \Big| \\
            & \propto \Big| \Big( I - \kalmangain \beljacob \Big) \Sigmab_{t+1|t} \Big| \\
            & \propto \Big| \Big( I - \Sigmab^{\frac{1}{2}} \Sigmab^{\frac{1}{2}} \beljacob^{\top}
                \big[\beljacob \Sigmab^{\frac{1}{2}} \Sigmab^{\frac{1}{2}} \beljacob^{\top} + \obscov_{t}\big]^{-1} \beljacob \Big) \Sigmab^{\frac{1}{2}} \Sigmab^{\frac{1}{2}} \Big| \\
            % & ~~~~~~~~~~~~~~~~~~~~~~~~~~~  + \obscov_{t}\big]^{-1} \beljacob \Big) \Sigmab^{\frac{1}{2}} \Sigmab^{\frac{1}{2}} \Big| \\
            & \propto \Big| \Big( I - \Sigmab^{\frac{1}{2}} \Sigmab^{\frac{1}{2}} \beljacob^{\top}
                \big[\beljacob \Sigmab^{\frac{1}{2}} \Sigmab^{\frac{1}{2}} \beljacob^{\top} + \obscov_{t}\big]^{-1} \beljacob \Big) \Sigmab^{\frac{1}{2}} \Sigmab^{\frac{1}{2}} \Big| \\
            & \propto \Big| \Big( I - \Sigmab^{\frac{1}{2}} \beljacob^{\top}
                \big[\beljacob \Sigmab^{\frac{1}{2}} \Sigmab^{\frac{1}{2}} \beljacob^{\top} + \obscov_{t}\big]^{-1} \beljacob \Sigmab^{\frac{1}{2}} \Big) \Big| \Big|\Sigmab^{\frac{1}{2}} \Sigmab^{\frac{1}{2}} \Big| \\
            % & \propto \Big| \Big( I - \mathsf{A}^{\top}
            %     \big[\mathsf{A}^{\top} \mathsf{A}^{\top} + \alpha I \big]^{-1} \mathsf{A}^{\top} \Big) \Big| \Big|\Sigmab^{\frac{1}{2}} \Sigmab^{\frac{1}{2}} \Big| \\
        \end{split}
    \end{equation}
    In this equation, it becomes evident that the only term influenced by our control actions at time $t$ is the observation Jacobian $\beljacob$, as $\Sigmab^{\frac{1}{2}}$ only depends on the estimation from the previous step.
}

    % where $\alpha$ represents the maximum expected observation noise. 
\flnote{
    Denoting $\mathsf{A} = \beljacob \Sigmab^{\frac{1}{2}}$, we can perform singular value decomposition (SVD)  
    where $D$ is a rectangular matrix with singular values $\lambda_{i}$ on its diagonal, $UU^{T} = U^{T}U = I$, and $QQ^{T} = Q^{T}Q = I$. 
    \begin{equation}
        \label{eqn:SVD}
        \begin{split}
            % \mathsf{A}  & = \beljacob \Sigmab^{\frac{1}{2}} = \mathsf{U} \mathsf{D} \mathsf{Q}^{\top} \\
            \mathsf{A}  & = \beljacob \Sigmab^{\frac{1}{2}} = U D Q^{\top} \\
        \end{split}
    \end{equation}
}

\flnote{
    % Using singular value decomposition (SVD) we can write $\mathsf{A}$ as $\mathsf{A} = U D Q^{T}$ where $D$ is a rectangular matrix with singular values $\lambda_{i}$ on its diagonal, $UU^{T} = U^{T}U = I$, and $QQ^{T} = Q^{T}Q = I$. 
    Substituting \eqref{eqn:SVD} into \eqref{eqn:entropy_} we get: 
    \begin{equation} \label{eqn:prod_eigenvals_derivation}
        \begin{split}
            &= |I - (UDQ)^{T}((UDQ)(UDQ)^{T} + \alpha I)^{-1}(UDQ) ||\Sigmab| \\
            &= |I - Q^{T}D^{T}U^{T}(UDQQ^{T}D^{T}U^{T} + \alpha I)^{-1}UDQ | |\Sigmab|\\
            &= |I - Q^{T}D^{T}U^{T}(UDD^{T}U^{T} + \alpha I)^{-1}UDQ ||\Sigmab| \\
            &= |Q^{T}Q - Q^{T}D^{T}U^{T}(UDD^{T}U^{T} + \alpha I)^{-1}UDQ ||\Sigmab| \\
            &= |Q^{T}||I - D^{T}U^{T}(UDD^{T}U^{T} + \alpha I)^{-1}UD | |Q||\Sigmab| \\
            &= |Q^{T}||Q||I - D^{T}U^{T}(UDD^{T}U^{T} + \alpha I)^{-1}UD | |\Sigmab|\\
            &= |I - D^{T}U^{T}(UDD^{T}U^{T} + \alpha I)^{-1}UD ||\Sigmab| \\
            &= |I - D^{T}U^{T}(UDD^{T}U^{T} + \alpha UU^{T})^{-1}UD ||\Sigmab| \\
            &= |I - D^{T}U^{T} U (DD^{T} + \alpha I)^{-1} U^{T}UD | |\Sigmab|\\
            &= |(I - D^{T}(DD^{T} + \alpha I)^{-1} D)| |\Sigmab|\\
        \end{split}
    \end{equation}
    \begin{equation} \label{eqn:prod_eigenvals}
        \entropy(\bel_{t+1}) = |\Sigmab| \prod_{i}^{N} \big(1 - \frac{\lambda_{i}^{2}}{\lambda_{i}^{2} + \alpha}\big) 
    \end{equation}
    Thus we show that the evolution of entropy is a function of the singular values of $\beljacob \Sigmab^{\frac{1}{2}}$. 
    From eq: \eqref{eqn:prod_eigenvals}, we see that a choice of $\beljacob$ that increases the magnitude of the singular values $\lambda_{i}$ of $\beljacob \Sigmab^{\frac{1}{2}}$ will decrease the entropy of the belief distribution. 
    Having shown the tie between the jacobian and decrease in entropy we must establish the connection the displacement of the tissue surface particles of the jacobian and show which choices of displacement will reduce entropy. 
    Showing these ties will demonstrate that our proposed heuristic of uncertainty weighted displacement will reduce entropy. 
}

% Meanwhile, we substitute $\obscov_{t}=\alpha I$,  We seek to understand how we can reduce entropy through our choice the jacobian $\beljacob$.
    
    % \begin{equation}
    %     \label{eqn:entropy_jacobian_relation}
    %     \begin{split}
    %         \entropy(\bel_{t+1}) & = \norm{\Sigma} \\
    %         &= |(I - K\beljacob) \Sigma| \\
    %         &= |\big( I - \Sigma \beljacob^{T} \big( \beljacob \Sigma \beljacob^{t} + \noisejacob \obscov \noisejacob^{T}\big)^{-1} \beljacob \big) \Sigma| \\
    %         &= | \Sigma - \Sigma \beljacob^{T} \big( \beljacob \Sigma \beljacob^{T} + \noisejacob \obscov \noisejacob^{T}\big)^{-1} \beljacob  \Sigma| \\
    %         &= | \Sigma - \Sigma \beljacob^{T} \big( \beljacob \Sigma^{\frac{1}{2}} \Sigma^{\frac{1}{2}} \beljacob^{t} + \noisejacob \obscov \noisejacob^{T}\big)^{-1} \beljacob  \Sigma| \\
    %         &= |\Sigma^{\frac{1}{2}}|\\
    %         &| I - \Sigma^{\frac{1}{2}} \beljacob^{T} \big( \beljacob \Sigma^{\frac{1}{2}} \Sigma^{\frac{1}{2}} \beljacob^{t} + \noisejacob \obscov \noisejacob^{T}\big)^{-1} \beljacob \Sigma^{\frac{1}{2}}|\\
    %         &|\Sigma^{\frac{1}{2}}| \\
    %         &= | I - \Sigma^{\frac{1}{2}} \beljacob^{T} \big( \beljacob \Sigma^{\frac{1}{2}} \Sigma^{\frac{1}{2}} \beljacob^{t} + \alpha I \big)^{-1} \beljacob \Sigma^{\frac{1}{2}}| |\Sigma|
    %     \end{split}
    % \end{equation}
    
    % \begin{equation} \label{eqn:entropy_jacobian_relation2}
    %     \begin{split}
    %         &= | I - \Sigma^{\frac{1}{2}} \beljacob^{T} \big( \beljacob \Sigma^{\frac{1}{2}} \Sigma^{\frac{1}{2}} \beljacob^{t} + V \big)^{-1} H  \Sigma^{\frac{1}{2}}| |\Sigmab|\\
    %         &= |I - A^{T}(AA^{T} + V)^{-1}A ||\Sigmab| \;, A = \beljacob \Sigma^{\frac{1}{2}} 
    %     \end{split}
    % \end{equation}
    
        % \item \textbf{Text: } In addition we also want to show what choice of displacement will reduce entropy and thus justify our proposed heuristic on uncertainty weighted displacement. 

    % Using Singular Value Decomposition we can write $A$ as $A = U D Q^{T}$ where $D$ is a rectangular matrix with singular values $\lambda_{i}$ on its diagonal, $UU^{T} = U^{T}U = I$, and $QQ^{T} = Q^{T}Q = I$. 
    % \begin{equation}
    %     \begin{split}
    %         &= |I - (UDQ)^{T}((UDQ)(UDQ)^{T} + \alpha I)^{-1}(UDQ) ||\Sigmab| \\
    %         &= |I - Q^{T}D^{T}U^{T}(UDQQ^{T}D^{T}U^{T} + \alpha I)^{-1}UDQ | |\Sigmab|\\
    %         &= |I - Q^{T}D^{T}U^{T}(UDD^{T}U^{T} + \alpha I)^{-1}UDQ ||\Sigmab| \\
    %         &= |Q^{T}Q - Q^{T}D^{T}U^{T}(UDD^{T}U^{T} + \alpha I)^{-1}UDQ ||\Sigmab| \\
    %         &= |Q^{T}||I - D^{T}U^{T}(UDD^{T}U^{T} + \alpha I)^{-1}UD | |Q||\Sigmab| \\
    %         &= |Q^{T}||Q||I - D^{T}U^{T}(UDD^{T}U^{T} + \alpha I)^{-1}UD | |\Sigmab|\\
    %         &= |I - D^{T}U^{T}(UDD^{T}U^{T} + \alpha I)^{-1}UD ||\Sigmab| \\
    %         &= |I - D^{T}U^{T}(UDD^{T}U^{T} + \alpha UU^{T})^{-1}UD ||\Sigmab| \\
    %         &= |I - D^{T}U^{T} U (DD^{T} + \alpha I)^{-1} U^{T}UD | |\Sigmab|\\
    %         &= |(I - D^{T}(DD^{T} + \alpha I)^{-1} D)| |\Sigmab|\\
    %     \end{split}
    % \end{equation}
    % \begin{equation} \label{eqn:prod_eigenvals}
    %     \entropy(\bel_{t+1}) = |\Sigmab| \prod_{i}^{N} \big(1 - \frac{\lambda_{i}^{2}}{\lambda_{i}^{2} + \alpha}\big) 
    % \end{equation}
    % Thus we show that the evolution of entropy is a function of the singular values of $\beljacob \Sigmab^{\frac{1}{2}}$. 
    % From eq: \ref{eqn:prod_eigenvals}, we see that a choice of $\beljacob$ that increases the magnitude of the singular values $\lambda_{i}$ of $\beljacob \Sigmab^{\frac{1}{2}}$ will decrease the entropy of the belief distribution. 
    % Having shown the tie between the jacobian and decrease in entropy we must establish the connection the displacement of the tissue surface particles of the jacobian and show which choices of displacement will reduce entropy. 
    % Showing these ties will demonstrate that our proposed heuristic of uncertainty weighted displacement will reduce entropy. 

    
    % ==============================================================
    % ==============================================================
    % ==============================================================
    % ==============================================================
    \textcolor{red}{moved to here!! todo} \\
    To convey the intuition behind this heuristic we look at the relationship between the change in entropy and the robot's actions. 
    We start by expanding \eqref{eqn:kalman_entropy} to express the evolution of entropy in terms of the kalman filter equations \eqref{eqn:update_step_multiple_shooting}. 
    \begin{equation}\label{eqn:entropy_kalman_expanded}
        \begin{split}
            & \entropy(\bel_{t+1}) \approxeq \\
            &ln\big(|\big( I - \Sigmab_{t} \beljacob_{t+1}^{T} \big( \beljacob_{t+1} \Sigmab_{t} \beljacob_{t+1}^{T} + \noisejacob_{t+1} \obscov_{t+1} \noisejacob_{t+1}^{T}\big)^{-1} \beljacob_{t+1} \big) \\
            &\Sigmab_{t}|\big) 
        \end{split}
    \end{equation}
    The Jacobian $\beljacob_{t+1}$, is the only term we can influence with our actions. 
    We substitute $\noisejacob_{t+1} = I$ and $\obscov_{t+1} = \alpha_{t} I$ from our observation model in \eqref{eqn:ekf_obs_model}, where $\alpha_{t}$ is the largest uniform observation noise variance: 
    \begin{equation}\label{eqn:entropy_singular_values}
        \begin{split}
            \entropy(\bel_{t+1}) \approxeq ln \big(|\Sigmab_{t}| \prod_{i}^{N} \big(1 - \frac{\lambda_{i}^{2}}{\lambda_{i}^{2} + \alpha}\big) \big),
        \end{split}
    \end{equation}
    where $\lambda_{i}$ are the singular values of $\beljacob_{t+1}\Sigmab^{\frac{1}{2}}$. 
    % As we increase the magnitude of $\lambda_{i}$ the product term decreases, approaching $0$. 
    Thus, in order to reduce entropy, we want to maximize the magnitude of the singular values of $\beljacob_{t+1}\Sigmab^{\frac{1}{2}}$.
weighted displacement will reduce entropy.
    To understand how our actions can affect $\beljacob_{t+1}\Sigmab^{\frac{1}{2}}$, we derive the jacobian $\beljacob_{t+1}$ using the implicit function theorem. 
    \begin{equation}\label{eqn:jacobian_implicit_function_thm}
        \begin{split}
            \beljacob_{t+1} = \jacBConstant(\bel_{t}) r(\Delta \statesim_{t+1})
        \end{split}
    \end{equation}
    \textcolor{notecolor}{NOTE: you might want mu in the notation above ?}
    $\jacBConstant(\bel_{t}) \in \mathbb{R}^{3n \times n}$ is a function of the current boundary belief $\bel_{t}$, but is constant with respect to tissue particle states.
    The direction displacement function $r(\Delta \statesim_{t+1})$ is defined in \eqref{eqn:r_matrix_definition}. 
    For details of the derivation and the explicit form of $J(\bel_{t})$ see section \textbf{REFERENCE} in the Appendix. 
    By \eqref{eqn:jacobian_implicit_function_thm} we see that that displacement directly controls the Jacobian $\beljacob_{t+1}$. 

    To minimize entropy we have to maximize the singular values of: $\jacBConstant(\bel_{t})r(\Delta \statesim_{t+1})\Sigmab^{\frac{1}{2}}$. 
    % To avoid the pitfalls of our entropy minimization metric, we aim to design a heuristic that reduces entropy independent of the current belief $\bel_{t}$.
    We choose a heuristic that is a function of $r(\Delta \statesim_{t+1})\Sigmab^{\frac{1}{2}}$, independent from $\jacBConstant(\bel)$ to avoid the pitfalls arising from excessive dependence on our current belief $\bel_{t}$. 
    % When there is no displacement, $r([\statesim_{t+1} - \stateref_{0}]) = 0$, $\Gamma = 0$, and all $\lambda_{i}^{2} = 0, \forall i$ resulting in no reduction in entropy. 
    % When there is non-zero displacement $r([\statesim_{t+1} - \stateref_{0}]) \neq 0$ resulting in $\lambda_{i}^{2} \geq 0, \forall i$. 
    When there is a non-zero displacement, $r(\Delta \statesim_{t+1}) \neq 0$, resulting in $\lambda_{i}^{2} \geq 0, \forall i$. 
    Thus we maximize our potential to decrease entropy when we increase the magnitude of displacement. 
    Inspired by the term $r(\Delta \statesim_{t+1})\Sigmab^{\frac{1}{2}}$ we choose to maximize the norm of $r(\Delta \statesim_{t+1})\Sigmab$. 
    Weighting the displacement with the current covariance matrix allows the heuristic to prioritize displacement and thus potential information gain in regions where the uncertainty in high. 

        
    % ==============================================================
    % ==============================================================
    % ==============================================================
    % ==============================================================

\flnote{
    \subsubsection{\textbf{Observation Jacobian Regarding the Uncertainty-Weighted Displacement (UWD)}}
    \textbf{Text: } In addition we also want to show what choice of displacement will reduce entropy and thus justify our proposed heuristic on uncertainty weighted displacement. 
}
    
    \begin{figure}[t]
        \centering
        % \includegraphics[width=0.9\linewidth]{images/PBD_structure_proof.png} 
        \includegraphics[width=0.6\linewidth]{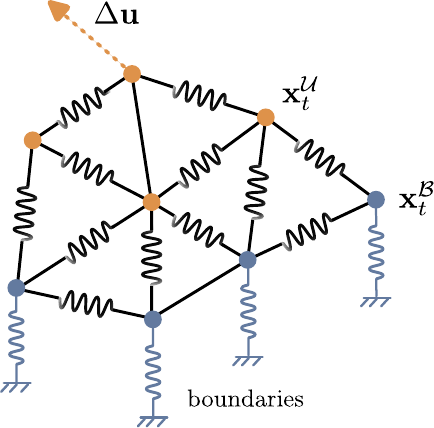} 
        \caption{PBD Structure for Proof}
        \label{fig:pbd_structure_proof}
    \end{figure}

    \subsection{Jacobian of PBD: Understanding the PBD simulator}  To derive the Jacobian: $\beljacob$ which is the jacobian of the PBD simulator with respect to the boundary constraints b, we start by understanding the PBD simulator. 
    In the PBD simulator the tissue is represented as a mesh consisting of particles connected to one another via constraints. 
    The constraints that parameterize our system are: $\proofBoundaryEnergy$ the boundary constraints, $\proofMeshEnergy$ the mesh constraints and $\proofActionEnergy$ the action or grasp constraints. 
    These capture the energy associated with the boundary, the mesh and the connection between the mesh and the grasp action particle respectively. 

    \textbf{NOTE: might want to specify why you divide things up}
        
    An example of the PBD constraint structure in the PBD is shown in figure \ref{fig:pbd_structure_proof}. 
    Here $a$ denotes a control particle that we can move to the desired location, this is connected to grasp particles $\ungraspedpts$ via the action constraints Cu. 
    These grasp particles do not have boundary connections that we are trying to estimate
    The grasp particles $\ungraspedpts$ are connected through the tissue mesh constraints, Cm, to some ungrasped particles $x^{u}_{t}$. 
    The ungrasped particles $x^{u}_{t}$ have constraints connecting them to the boundary and are parameterized by the $b$ that we are estimating. 
    Thus we divide our tissue state representation $x_{t}$ into ungrasped and grasped particles for our derivation such that $x_{t} = \fullstatepts$. 
    Let us assume there are $n$ ungrasped particles and $m$ grasped particles. 
    $b \in \mathbb{R}^{n}$ as there are $n$ boundary constraint parameter associated with $n$ ungrasped particles to estimate. 
    $x_{t} \in \mathbb{R}^{3(n +m) \times 1}$ is a flattened vector of the 3 dimensional particle states of size  and thus $\graspedpts \in \mathbb{R}^{3n \times 1}$, $\ungraspedpts \in \mathbb{R}^{3m \times 1}$.
        
    \textbf{Equation: } All the constraint equations
    \begin{equation} \label{eqn:pbd_boundary_constraint}
        \begin{split}
            \proofBoundaryEnergy(\ungraspedpts, b) = \frac{1}{2} [\ungraspedpts - x^{u}_{0}]^{T}B[\ungraspedpts - x^{u}_{0}] 
        \end{split}
    \end{equation}
    $\graspedpts - x^{u}_{0}$ is the displacement of the ungrasped particles at time $t$ from their original positions at time $t=0$. 
    $B \in \mathbb{R}^{3n \times 3n}$ is a diagonal matrix where each boundary constraint parameter is repeated $3$ times along the diagonal: $B[3i, 3i]=b[i], B[3i+1, 3i+1]=b[3i+1], B[3i+2, 3i+2]=b[3i+2]$. 
    This construction of $B$ is as the energy associated with boundary constraint parameter associated with particle $i$ is impacted by $3$ dimensions of the particle position. 
        
    \begin{equation} \label{eqn:pbd_mesh_constraint}
        \begin{split}
            \proofMeshEnergy(x_{t}) = x_{t}^{T} L x_{t} - x^{T} J q
        \end{split}
    \end{equation}
    $L \in \mathbb{R}^{3(m+n) \times 3(m+n)}$ captures the connections and constraints between all grasped and ungrasped particles in the mesh. 
    \textbf{NOTE: ADD WHAT J AND q mean}
        
    \begin{equation} \label{eqn:pbd_grasp_constraint}
        \begin{split}
            \proofActionEnergy(\ungraspedpts, a_{t}) = [\ungraspedpts - \hat{a_{t}}]^{T} K [\ungraspedpts - \hat{a_{t}}]
        \end{split}
    \end{equation}
    $\hat{a_{t}} \in \mathbb{R}^{3m \times 1}$ is a vector of the 3 dimensional action point stacked $m$ times. 
    $[\ungraspedpts - \hat{a}]$ denotes the displacement between the action point $a$ and the grasped particles $\ungraspedpts$. 
    $K = k I \in \mathbb{R}^{3m \times 3m}, k \in \mathbb{R}$ denotes the fixed spring constraint used to connect the action particle $a$ to the grasped particles $x^{t}_{t}$. 
        
    Together these constraints provide equations provide a function for the energy of the tissue as a function of the tissue surface particles for a given action $a_{t}$.
    \begin{equation}
        \energy(x_{t}) = \proofBoundaryEnergy(\graspedpts, b) +  \proofMeshEnergy(x_{t}) +  \proofActionEnergy(\ungraspedpts, a_{t})
    \end{equation}
    As stated in section REFERENCE, the PBD simulator solves for the next state of the tissue surface particles by iteratively updating the particles to minimize the energy in the system. 
    The PBD can be summarized using the following equation: 
    \begin{equation} \label{eqn:pbd_argmin_energy}
        x_{t} = \arg\min_{x_{t}} = \energy(x_{t}, b)
    \end{equation}

    \subsection{Jacobian of PBD: Implicit Function Theorem Setup} To get the jacobian, $\beljacob$, of the next state $x_{t}$ outputted by the PBD simulator with respect to the boundary function parameters b, we use the implicit function theorem. 
    The Implicit function theorem states that given a stationary Function $F(x_{t}, b)$ that gives the relationship between 2 variables $x_{t}$ and $b$, we have an implicit function $x_{t} = g(b)$ in the neighborhood of some $x_{t}$ whose jacobian $\frac{dg(b)}{db}$ is given by:  $\frac{dg(b)}{db} = -{\frac{dF(g(b), b)}{dx_{t}}}^{-1} \frac{dF(g(b), b)}{db}$. 
    This holds assuming we have a relationship function $F$ such that $F(x_{t}, b) = 0$ in the neighborhood $(x_{t}, b)$ that we evaluating near and if the jacobian $\frac{dF(g(b), b)}{dx_{t}}$ is invertible. 
    We choose the jacobian of our energy function with respect to the tissue particle state $x_{t}$ as our relationship function $F=\frac{d \energy(x_{t}, b)}{d x_{t}}$. 
    The state $x_{t}$ that we are evaluating near is the output of the PBD at the $\arg\min_{x_{t}} \energy(x_{t}, b)$ for the current boundary constraint value $b$.  
    As $\energy(x_{t}, b)$ is quadratic $\frac{d \energy(x_{t}, b)}{d x_{t}} = 0$ at the state outputted from the PBD. 
    As we can numerically compute the jacobian through the PBD we assume that $\frac{dF(g(b), b)}{dx_{t}} = \frac{d^{2} \energy}{d x_{t}^{2}}$ is invertible and thus the jacobian can be computed. 

    \subsection{Jacobian of PBD: Implicit Function Theorem Solution} Using our choice of $F=\frac{d \energy(x_{t}, b)}{d x_{t}}$, we solve for the jacobian $\beljacob = -{\frac{dF(g(b), b)}{dx_{t}}}^{-1} \frac{dF(g(b), b)}{db} = - {\frac{d^{2} \energy}{d x_{t}^{2}}}^{-1} \frac{d \energy}{db dx_{t}}$. 
    We start by solving for ${\frac{d^{2} \energy}{d x_{t}^{2}}}$. 
    We denote $x_{t} = \fullstatepts$ giving us: 
        
    $\displaystyle {\frac{d^{2} \energy}{d x_{t}^{2}}} = {\frac{d^{2} \energy}{d \fullstatepts^{2}}} \in \mathbb{R}^{3(n+m) \times 3(n+m)}$
    \begin{equation} \label{eqn:d2U_dx2}
        \begin{split}
            &\frac{d \energy}{d \fullstatepts} 
            = \begin{bmatrix}
                \frac{d \proofBoundaryEnergy}{d \ungraspedpts} + \frac{d \proofMeshEnergy}{d \ungraspedpts} \\
                \frac{d \proofMeshEnergy}{d \graspedpts} + \frac{d \proofActionEnergy}{d \graspedpts}
                \end{bmatrix} \\
            %
            &\frac{d^{2} \energy}{d \fullstatepts^{2}} 
            = \begin{bmatrix}
                \frac{d^{2} \proofBoundaryEnergy}{d \ungraspedpts^{2}} + \frac{d^{2} \proofMeshEnergy}{d \ungraspedpts^{2}} & 
                \frac{d \proofMeshEnergy}{d\graspedpts d \ungraspedpts} \\    
                \frac{d \proofMeshEnergy}{d\ungraspedpts d \graspedpts} & 
                \frac{d^{2} \proofMeshEnergy}{d \graspedpts^{2}} + \frac{d^{2} \proofActionEnergy}{d \graspedpts^{2}}
                \end{bmatrix}
        \end{split}
    \end{equation}

    Plugging in the values we get: 
    \begin{equation} \label{eqn:filled_d2U_dx2}
        \begin{split}
            &\frac{d^{2} \energy}{d \fullstatepts^{2}} 
            = \begin{bmatrix}
                B + 2L_{u,u} & L_{u,g} + L_{g,u}^{T} \\
                L_{g,u} + L_{u,g}^{T} & 2L_{g,g} + K
            \end{bmatrix} \\
            &L = \begin{bmatrix}
                L_{u,u} & L_{u,g} \\
                L_{g,u} & L_{g,g}
            \end{bmatrix} 
        \end{split}    
    \end{equation}
    % $L_{u, u} = L[0:3n, 0:3n] \in \mathbb{R}^{3n \times 3n}, L_{m, m} = L[3n:3(n+m), 3n:3(n+m)] \in \mathbb{R}^{3m \times 3m}$ and $L_{u, g} = L[0:3n, 3n:3(n+m)] \in \mathbb{R}^{3n \times 3m}, L_{g,u} = L[3n:3(n+m), 0:3n)] \in \mathbb{R}^{3m \times 3n}$. 
    $B$ and $K$ are as defined above. 

    We Now solve for $\frac{d \energy}{db dx_{t}}$:
    \begin{equation}\label{eqn:dU_dbdx}
        \frac{d \energy}{db dx_{t}} 
        = \begin{bmatrix}
            \frac{d \proofBoundaryEnergy}{d b d\ungraspedpts} \\
            0 
        \end{bmatrix} \\
        = \begin{bmatrix}
            \frac{d B [\ungraspedpts - x^{u}_{0}] }{d b} \\
            0
        \end{bmatrix}
        = \begin{bmatrix}
            r([\ungraspedpts - x^{u}_{0}]) \\
            0
        \end{bmatrix}
    \end{equation}

    Here $r([\ungraspedpts - x^{u}_{0}]) \in \mathbb{R}^{3(n) \times n}$ is a matrix that is a direct function of displacement of the ungrasped particles $\ungraspedpts - x^{u}_{0}]$ and $0 \in \mathbb{R}^{3m \times n}$
    In Column $i$ of $r([\ungraspedpts - x^{u}_{0}])$ indices $3i, 3i+1, 3i+2$ correspond to the displacement of ungrasped particle $i$: $r([\ungraspedpts - x^{u}_{0}])[3i:3i+3, i] = [\ungraspedpts - x^{u}_{0}][3i:3i+3]$. 
    % \begin{equation} \label{eqn:r_matrix_definition}
    %     \begin{split}
    %         &r([\ungraspedpts - x^{u}_{0}]) = \\
    %         &\begin{bmatrix}
    %             \ungraspedpts^{,0} - x^{u, 0}_{0} & 0 & 0& \cdots & 0\\
    %             0 & \ungraspedpts^{,1} - x^{u, 1}_{0} & 0 & \cdots & 0\\
    %             \vdots & \vdots &  \vdots & \ddots & \vdots \\
    %             0 & 0 & 0 & \cdots & \ungraspedpts^{,n-1} - x^{u,n-1}_{0}
    %         \end{bmatrix}
    %     \end{split}
    % \end{equation}
    \begin{equation} \label{eqn:r_matrix_definition_2}
        \begin{split}
            &r([\ungraspedpts - x^{u}_{0}]) = \\
            &\begin{bmatrix}
                \ungraspedpts^{,0} - x^{u, 0}_{0} & 0 & \cdots & 0\\
                0 & \ungraspedpts^{,1} - x^{u, 1}_{0} & \cdots & 0\\
                \vdots & \vdots & \ddots & \vdots \\
                0 & 0 & \cdots & \ungraspedpts^{,n-1} - x^{u,n-1}_{0}
            \end{bmatrix}
        \end{split}
    \end{equation}
        
    % \begin{equation} \label{eqn:r_matrix_definition}
    %     \begin{split}
    %         &r([\ungraspedpts - x^{u}_{0}]) = \\
    %         &\begin{bmatrix}
    %             \ungraspedpts^{,0} - x^{u, 0}_{0} & 0 & 0\\
    %             0 & &  \\
    %             \vdots & \ddots & \vdots \\
    %             0 & \cdots & 0 \> \> \ungraspedpts^{,n-1} - x^{u,n-1}_{0}
    %         \end{bmatrix}
    %     \end{split}
    % \end{equation}
    Here $\ungraspedpts^{,i} - x^{u, i}_{0} \in \mathbb{R}^{3}$ denotes the $3$ dimensional displacement of ungrasped particle $i$ of the tissue surface at time $t$ from its original position at $t=0$.  
        
    For example if we considered the case where there was just one ungrasped particle: 
    \begin{equation}
       \begin{bmatrix}
            r([\ungraspedpts - x^{u}_{0}]) \\
            0
        \end{bmatrix} 
        = \begin{bmatrix}
            [\ungraspedpts - x^{u}_{0}] \\
            0
        \end{bmatrix}
    \end{equation}
    which is exactly displacement. 

    With this we get that the jacobian $\beljacob$ is: 
    \begin{equation}
        \begin{split}
            \beljacob = -{\frac{d^{2} \energy}{d \fullstatepts^{2}}}^{-1} \frac{d^{2} \energy}{db d \fullstatepts}\\
            = -1 \begin{bmatrix}
                B + 2L_{u,u} & L_{u,g} + L_{g,u}^{T} \\
                L_{g,u} + L_{u,g}^{T} & 2L_{g,g} + K
            \end{bmatrix}^{-1} 
            \begin{bmatrix}
                r([\ungraspedpts - x^{u}_{0}]) \\
                0
            \end{bmatrix}
        \end{split}
    \end{equation}

    Note that the first term in this is a function of the current boundary parameter belief $\bel$, but it just a constant with respect to the tissue surface particle states. 
    Going forward we will refer to going forward as $\jacBConstant(\bel) = -{\frac{d^{2} \energy}{d \fullstatepts^{2}}}^{-1}$. 
    As a result we get that $\beljacob$ is a direct function of the displacement of the ungrasped tissue particles whose boundary connection parameters, $b$, we are estimating. 

    \subsection{Choosing Displacement to Reduce Entropy: } Tying this to the formula for entropy we get that the change in entropy is related to the singular values of: 
    \begin{equation}
        \beljacob \Sigmab^{\frac{1}{2}} 
        = \jacBConstant(\bel) \begin{bmatrix}
                    r([\ungraspedpts - x^{u}_{0}]) \\
                    0
                \end{bmatrix} 
                \Sigmab^{\frac{1}{2}}
    \end{equation}
    Thus the reduction in entropy is a direct function of the displacement of the tissue surface particles that we can control 
    To consider how to control displacement to reduce entropy we consider the case where we are trying to estimate the boundary connection parameter $b$ for a single ungrasped particle. 
    Here we get that:  
    \begin{equation}
        \beljacob \Sigmab^{\frac{1}{2}} 
        = \jacBConstant(\bel) \begin{bmatrix}
            [\ungraspedpts  - x^{u}_{0} ]\\
            0 
        \end{bmatrix}
        \sigma^{\frac{1}{2}}
    \end{equation}
    Here $[\ungraspedpts  - x^{u}_{0} ]$ is the displacement of the ungrasped particle whose boundary connection parameter we want to estimate and $\sigma^{\frac{1}{2}} \in \mathbb{R}$ and $J \in \mathbb{R}^{3(n+m) \times 3(n+m)}$ is a constant matrix. 
    The singular value of this matrix is a scalar $\lambda$: 
    \begin{equation}
        \lambda = \sqrt{\sigma 
        \begin{bmatrix}
            [\ungraspedpts  - x^{u}_{0} ]^{T} & 0
        \end{bmatrix}^{T}
        \jacBConstant(\bel)^{T}\jacBConstant(\bel) 
        \begin{bmatrix}
            [\ungraspedpts  - x^{u}_{0} ] \\
            0
        \end{bmatrix}
        }
    \end{equation}
    Here you can see that if displacement is $0$ the singular value $\lambda$ goes to $0$ meaning there will be no reduction in entropy. 
    With non-zero displacement on the particle where we are estimating $b$ we ensure that the $\lambda \geq 0$, thus relating non-zero displacement to a decrease in entropy of our belief distribution. 
    This intuition informs our heuristic choice using maximum displacement. 

    For multiple particles the singular values $\lambda_{i}, i\in[0, N-1]$ are the eigenvalues of matrix $\Gamma$: 
    \begin{equation}
        \Gamma = \Sigmab^{\frac{1}{2}}
        \begin{bmatrix}
            r([\ungraspedpts  - x^{u}_{0} ])^{T} & 0
        \end{bmatrix}^{T}
        \jacBConstant(\bel)^{T}\jacBConstant(\bel) 
        \begin{bmatrix}
            [\ungraspedpts  - x^{u}_{0} ] \\
            0
        \end{bmatrix}
        \Sigmab^{\frac{1}{2}}
    \end{equation}
    As in the single particle case if our displacement at all the ungrasped particles is $0$, $\Gamma = 0$ causing $\lambda_{i} = 0, \forall i$. 
    Thus we want to ensure we have non-zero displacement. 
    Particularly in effort to maximize the eigenvalues of $\Gamma$ we seek to maximize displacement in the direction weighted most by uncertainty, inspired by the term: $\begin{bmatrix}
                [\ungraspedpts  - x^{u}_{0} ] \\
                0
            \end{bmatrix}
            \Sigmab^{\frac{1}{2}}$. 
    \textbf{NOTE: MIGHT WANT TO SWAP OUT DEPENDING ON WHICH HEURISTIC YOU ACTUALLY END UP USING!}
    This informs our heuristic function of uncertainty weighted displacement where we aim to maximize the norm of the displacement of particles weighted by the variance values of our belief at those particle locations. 


\subsection{Pre-defined Motion Primitives}\label{appendix:predefined_motion_primitives}


% \subsection{Active Sensing Framework: \textbf{NOTE:From OLD active sensing, Delete this after looking over it again}}

% \begin{itemize}
%     \item We can use our belief on the structure of the tissue, from our estimation framework, to guide which actions we can take for optimal discovery of the tissue structure. 
%     \begin{itemize}
        
%         \item As our belief on the boundary connections is formulated as a probability distribution, we seek to take the actions that will lead to the minimization of the entropy of our belief distribution. 

%         \item The entropy of a gaussian distribution is 
%         \begin{equation}
%             \entropy(\bel_{t+1}) = \frac{D}{2}(1 + ln(2 \pi)) + ln(|\Sigmab_{t+1|t}|)
%         \end{equation}
%         Here $D$ is the dimensionality of the multivariate gaussian distribution. 
%         We use this to find the best action to take to minimize entropy $\arg\min_{\action_{t}} \entropy(\bel_{t+1}) = \arg\min_{\action_{t}} ln(|\Sigmab_{t+1|t}|)$. 

%         \item Given a control and the Kalman filter equations we express evolution of entropy as a function of the action, allowing us to re-phrase the minimization as: 
%         \begin{equation} \label{eqn:minimize_entropy}
%             \begin{split}
%                 \arg\min_{\action_{t} \in \mathcal{U}}ln(|\entropy(\bel_{t+1})|) \; \\ 
%                 s.t. \; \boundaryenergy(\bel_{t+1}) \leq E_{\max}, \inworkspace(\action_{t}) \leq \inworkspace_{\max}
%             \end{split}
%         \end{equation}

%         \begin{equation} \label{eqn:minimize_entropy_kalman}
%             \begin{split}
%             \arg\min_{\action_{t} \in \mathcal{U}} ln \big( |(I - K_{t+1|t} \beljacob_{t+1}) \Sigmab_{t+1} |\big) \\
%             s.t. \; \boundaryenergy(\bel_{t+1}) \leq E_{\max}, \inworkspace(\action_{t}) \leq \inworkspace_{\max}
%             \end{split}
%         \end{equation}
%         % \Sigma_{t+1|t} H_{t+1} (H_{t+1} \Sigma_{t+1|t} H_{t+1}^{T} + R_{t+1}V_{t+1}R_{t+1}^{T})^{-1}
%         Here $\beljacob_{t+1}$ and $K_{t+1}$ are functions of the action $\action_{t}$.

%         \item Using this we formulate the following loss to minimize and find actions for local feedback control: 
%         % \begin{equation} \label{eqn:feedback_entropy_loss}
%         %     \begin{split}
%         %         \arg\min_{u_{t}} l(u_{t}, b_{t}, x_{ref, t}) = ln \big( |(I - K_{t+1|t} H_{t+1}) \Sigma_{t+1} |\big) + \\
%         %         de(b_{t}) + iw(u_{t})
%         %     \end{split}
%         % \end{equation}

%         \begin{equation}\label{eqn:feedback_entropy_loss}
%             \begin{split}
%                  \Delta \action = - \nabla_u \entropy(\bel_t) - 
%                 \nabla_\action \boundaryenergy(\bel_{t}) - \nabla_\action \inworkspace(\action_{t})
%             \end{split}
%         \end{equation}

%         \item In addition to entropy minimization we want to prevent excessive unsafe deformation along the boundary by also minimizing the deformation energy along the current known boundary, $\boundaryenergy(\bel_{t}, \action_{t}, \stateref_{, t})$, after action $\action_{t}$ in our loss term. 

%         \item Additionally the term $\inworkspace(u_{t})$ is the in workspace loss which penalizes actions that cause the grasp point to exit a set constraint workspace. 

%         \item We can find the action that locally minimizes this loss function to greedily compute local feedback control. 

%         \item To do this we compute the loss for a candidate action from the current state. 

%         \item Since the PBD simulator and every component of our framework is differentiable, we can then compute a gradient, $\frac{d l(\action_{t}, \bel_{t}, \stateref_{, t})}{d \action_{t}}$, which we use to update our action $\action_{t}$.

%         \item After optimizing we can take an action, use the new observation in conjunction with our estimation framework to update our belief, $\mub_{t+1}, \Sigmab_{t+1}$ and then re-optimize our control and repeat this process.  

%         \item Doing this at every step we get a local feedback controller that greedily takes actions to decrease entropy while minimizing boundary deformations and workspace violations with each step, 

%         \item \textbf{We might want to add a discussion of when we want to stop finding actions ? eg if there is no decrease in entropy after a given number of steps stop, or that technically things should stop by themself ?: } With this approach we can pose a stopping condition when the entropy fails to decrease beyond a certain amount over a fixed number of steps, though in practice as the loss function fails to find entropy minimizing actions it should seize to move the tissue as doing so will only incur a penalty via the other losses. 
%     \end{itemize}

%     \item Entropy based feedback control can be slow to compute over repeated iterations due to speed of the jacobian computation in the kalman filter update step required to evaluate the propagation of entropy. 
%     \begin{itemize}
%         \item To address the computational complexity of this method we develop another heuristic based loss metric with the same goal of decreasing the entropy in our belief distribution to maximize information gain. 

%         \item The heuristic we choose is the maximization of the displacement of each of the tissue vertices from their original resting positions weighted by the uncertainty of the current belief, denoted by  $\displacement(\stateref_{, t}, \action_{t}, \bel_{t})$: 
%         \begin{equation} \label{eqn:probabilistic_displacement_loss}
%             \begin{split}
%                  \displacement(\stateref_{, t}, \action_{t}, \bel_{t}) = \\
%                  \frac{1}{N}\Sigma_{i=0}^{N} \Sigmab_{t}[i, i] \\
%                  || \statesim_{0}[i] - \pbd(\stateref_{, t}, \action_t, \mub_{t})[i]||_{2}
%             \end{split}
%         \end{equation}
%         For this heuristic loss we take the uncertainty weighted norm of the displacement of each expected tissue surface particle from its resting position. 

%         \item As a result we seek out larger displacement in regions that remain uncertain. 

%         \item We use this heuristic to formulate a loss that we minimize: 
%         % \begin{equation}\label{eqn:feedback_displacement_loss}
%         %     \begin{split}
%         %         \arg\min_{u_{t}} l(u_{t}, b_{t}, x_{ref, t}) = -ud(x_{ref, t}, u_{t}, b_{t}) \\ 
%         %         + de(b_{t}) + iw(u_{t})
%         %     \end{split}
%         % \end{equation}

%         \begin{equation}\label{eqn:feedback_displacement_loss}
%             \begin{split}
%                 \Delta \action = \nabla_\action \displacement(\stateref_{, t}, \action_{t}, \bel_{t}) 
%                 - \nabla_\action \boundaryenergy(\bel_{t}) -\nabla_\action \inworkspace(\action_{t})
%             \end{split}
%         \end{equation}

%         \item As with entropy based feedback control we use a gradient step on the loss to optimize our actions before taking a step, updating our belief and repeating the process. 
%     \end{itemize}

%     \item To explain our choice of heuristic we consider a simple single particle spring system. 
%     \begin{itemize}
%         \item In this system a single particle is attached to a fixed ground location using a zero length boundary constraint spring with stiffness $\bel$. 
%         \item This system is governed by the equation $F = -\bel x$ where $F$ is the force exerted by the spring when the particle is displaced from its resting position by $x$. 
%         \item From this we have that $x = -\frac{F}{\bel}$. 
%         \item The PBD uses this sort of mass spring model and iteratively solves these equations to compute the particle displacements $x$. 
%         \item From this equation we also get the jacobian $\frac{d x}{d \bel} = \frac{F}{\bel^{2}}$
%         \item As we are considering quasi-static scenarios where the system is in equillibrium, the force, $F$, exerted by the spring is equal to the external force. 
%         \item Thus when there is no displacement in the particle the force exerted by the spring is $0$, leading the jacobian with respect to $b$ to also be $0$. 
%         \item When there is displacement the particle is being held by an external non-zero force, matched by the spring, resulting in a non-zero jacobian with respect to $\bel$. 
%         \item Intuitively this means that in a situation where the particle would be displaced, changing the value of $\bel$ would have an impact on the observed simulation, thus yielding more information about the value of $\bel$ at that particle. 
%     \end{itemize}

%     \item To demonstrate that this heuristic results in decreasing entropy of our belief we analyze the relationship between the jacobian $\beljacob_{t+1}$, and the evaluation of entropy via the kalman filter. 
%     \begin{itemize}
%         \item To do this we start by looking at the the equation for entropy of the boundary connections estimated by our Kalman Filter \ref{eqn:feedback_entropy_loss}. 
%         For the purposes of this derivation we will refer to $\beljacob_{t+1} = \beljacob, K_{t+1|t} = K, \Sigmab_{t+1|t} = \Sigma, \noisejacob_{t+1} = \noisejacob, \obscov_{t+1} = \obscov$. 
%         \begin{equation} \label{eqn:entropy_jacobian_relation}
%             \begin{split}
%                 & E(\bel_{t+1}) = |\Sigmab_{t+1|t+1}| \\
%                 &= |(I - K\beljacob) \Sigma| \\
%                 &= |\big( I - \Sigma \beljacob^{T} \big( \beljacob \Sigma \beljacob^{t} + \noisejacob \obscov \noisejacob^{T}\big)^{-1} \beljacob \big) \Sigma| \\
%                 &= | \Sigma - \Sigma \beljacob^{T} \big( \beljacob \Sigma \beljacob^{T} + \noisejacob \obscov \noisejacob^{T}\big)^{-1} \beljacob  \Sigma| \\
%                 &= | \Sigma - \Sigma \beljacob^{T} \big( \beljacob \Sigma^{\frac{1}{2}} \Sigma^{\frac{1}{2}} \beljacob^{t} + \noisejacob \obscov \noisejacob^{T}\big)^{-1} \beljacob  \Sigma| \\
%                 &= |\Sigma^{\frac{1}{2}}|\\
%                 &| I - \Sigma^{\frac{1}{2}} \beljacob^{T} \big( \beljacob \Sigma^{\frac{1}{2}} \Sigma^{\frac{1}{2}} \beljacob^{t} + \noisejacob \obscov \noisejacob^{T}\big)^{-1} \beljacob \Sigma^{\frac{1}{2}}|\\
%                 &|\Sigma^{\frac{1}{2}}| \\
%             \end{split}
%         \end{equation}
%         We can break $\Sigma$ into $\Sigma^{\frac{1}{2}}\Sigma^{\frac{1}{2}}$ as $\Sigma$ is a positive semidefinite matrix. 
%         Since we are ultimately trying to minimize entropy with respect to the action $\action_{t}$ and thus only care about the relationship between entropy and $\beljacob_{t+1}$, we can disregard constant terms such as those relating to $\Sigma^{\frac{1}{2}}$. 
%         In our case $\noisejacob = I$, and $\obscov$ is a diagonal noise covariance matrix. 
%         \begin{equation} \label{eqn:entropy_jacobian_relation2}
%             \begin{split}
%                 &= | I - \Sigma^{\frac{1}{2}} \beljacob^{T} \big( \beljacob \Sigma^{\frac{1}{2}} \Sigma^{\frac{1}{2}} \beljacob^{t} + V \big)^{-1} H  \Sigma^{\frac{1}{2}}| \\
%                 &= |I - A^{T}(AA^{T} + V)^{-1}A | \;, A = \beljacob \Sigma^{\frac{1}{2}} 
%             \end{split}
%         \end{equation}
%         Using Singular Value Decomposition we can write $A$ as $A = U D Q^{T}$ where $D$ is a rectangular matrix with singular values $\lambda_{i}$ on its diagonal, $UU^{T} = U^{T}U = I$, and $QQ^{T} = Q^{T}Q = I$. 
%         \begin{equation}
%             \begin{split}
%                 &= |I - (UDQ)^{T}((UDQ)(UDQ)^{T} + \obscov)^{-1}(UDQ) | \\
%                 &= |I - (UDQ)^{T}(UDQQ^{T}D^{T}U^{T} + \obscov)^{-1}(UDQ) | \\
%                 &= |I - (UDQ)^{T}(UDD^{T}U^{T} + \obscov)^{-1}(UDQ) | \\
%                 &= |I - Q^{T}D^{T}U^{T}(UDD^{T}U^{T} + \obscov)^{-1}(UDQ) | \\
%                 &= |I - Q^{T}D^{T}U^{T}(UDD^{T}U^{T} + \obscov)^{-1}UDQ | \\
%                 &= |Q^{T}Q - Q^{T}D^{T}U^{T}(UDD^{T}U^{T} + \obscov)^{-1}UDQ | \\
%                 &= |Q^{T}||I - D^{T}U^{T}(UDD^{T}U^{T} + \obscov)^{-1}UD | |Q| \\
%                 &= |Q^{T}||Q||I - D^{T}U^{T}(UDD^{T}U^{T} + \obscov)^{-1}UD | \\
%                 &= |I - D^{T}U^{T}(UDD^{T}U^{T} + \obscov)^{-1}UD | \\
%             \end{split}
%         \end{equation}
%         \textbf{Can we show this with general diagonal V ? I don't think so ?}
%         We change the noise matrix $\obscov = \alpha I$ where $\alpha$ is a constant denoting the upper bound on the noise. \textbf{Make sure you want to use upper bound ?, might just want to change this to be an assumption we make instead of justifying it ?}
%         \begin{equation}
%             \begin{split}
%                 &= |I - D^{T}U^{T}(UDD^{T}U^{T} + \alpha I)^{-1}UD | \\
%                 &= |I - D^{T}U^{T}(UDD^{T}U^{T} + \alpha UU^{T})^{-1}UD | \\
%                 &= |I - D^{T}U^{T} U (DD^{T} + \alpha I)^{-1} U^{T}UD | \\
%                 &= |(I - D^{T}(DD^{T} + \alpha I)^{-1} D)| \\
%                 &= \prod_{i}^{N} 1 - \frac{\lambda_{i}^{2}}{\lambda_{i}^{2} + \alpha}
%             \end{split}
%         \end{equation}

%         From this derivation we see that the evolution of entropy is related to the magnitude of the singular values $\lambda_{i}$ of $H\Sigma^{\frac{1}{2}}$ which jacobian weighted by the uncertainty or the covariance matrix. 

%         \item A high magnitude of $\lambda_{i}^{2}$ in comparison to the noise term $\alpha$ results in $\frac{\lambda_{i}^{2}}{\lambda_{i}^{2} + \alpha}$ approaching 1 causing the product to approach $0$ and entropy to decrease. 

%         \item This translates to choosing a jacobian with high singular values or high impact in the direction of uncertainty, or the eigenvectors of the covariance matrix, results in a reduction of entropy. 

%         \item As higher magnitude values in the jacobian matrix are correlated with large displacement and by weighting displacement to prioritize regions of high uncertainty, our probabilistic displacement heuristic helps result in the reduction in entropy of our belief. 
%     \end{itemize}



%     \item Fig. \ref{fig:large_step_prediction}. Though the feedback control based approaches decrease entropy, they are susceptible to local minima and fail to consider longer term actions that allow more intricate maneuvers to gain information in these complex deformable environments. 
%     \begin{itemize}
%         \item To address this we develop a new approach where we intelligent sample several long range actions. 
%         \item We then compute the probabilistic displacement loss after forward simulating from the current state to these sampled long range target grasp points. 
%         \item Using gradient steps we optimize the final location of each of these long range target grasps. 
%         \item Then we take a step in the direction of the target grasp point with the lowest probabilistic displacement loss. 
%         \item We repeat this sampling and optimization procedure after each step with the updated belief distribution. 
%         \item Considering these long range actions allows us to decrease entropy by getting out of local minima. 
%         \item Though a similar approach would be feasible using our entropy loss from equation \ref{eqn:feedback_entropy_loss}, it is computationally prohibitive to do so due to the computational complexity of parallely computing multiple jacobians of our simulation. 
%     \end{itemize}

%     % later
%     % \item We extend this active sensing approach to consider environments that are changing such as after toplogy altering events like cuts and sutures.     

    
% \end{itemize}
